# Supplementary material for: Oxidized silicon sulfide: stability and electronic properties of a novel two-dimensional material
Source: arXiv:1904.09614 source file (2019-04-21)
Supplement: Supplementary file 1 [file SiSO18-SM.pdf]

# Supplemental on-line material for:
# Oxidized silicon sulfide: stability and electronic properties of a novel two-dimensional material

Zhengnan Li, Shuai Dong, and Jie Guan*

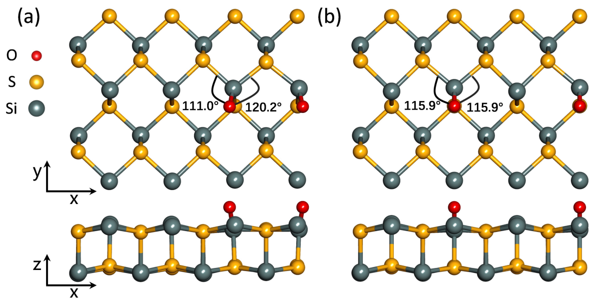


FIG. S1. Ball-and-stick model in the top view and side view of equilibrium structures for two oxygen atoms absorbed on (a) neighboring and (b) spaced Si atoms in $\alpha$-SiS. The S-Si-O bond angles are marked in the top view.

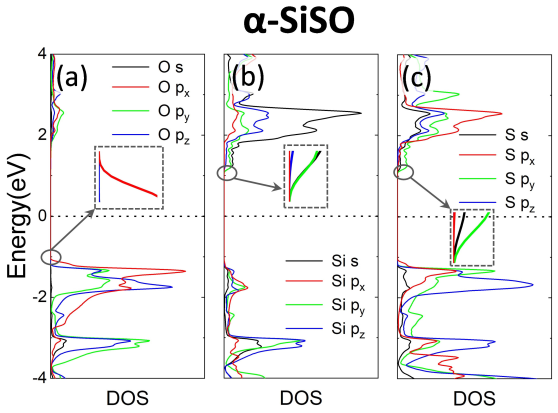


FIG. S2. Projected density of states (PDOS) of different orbitals from (a) O, (b) Si and (c) S in $\alpha$-SiSO monolayer. Contributions of electrons from different orbitals are distinguished by color. A figure zoomed in near the valence band maximum (VBM) is shown as inset in (a). Figures zoomed in near the conduction band minimum (CBM) are shown as insets in (b) and (c).

## INTERACTION BETWEEN O ATOMS ABSORBED ON $\alpha$-SiS

As mentioned in the main manuscript, the binding energy $E_b$ per oxygen atom for the fully optimized $\alpha$-SiS (2.70 eV) is a little smaller than that for the isolated oxygen impurity (2.92 eV). To reveal the reason for this, situations of two oxygen atoms absorbed on neighboring and spaced Si atoms in $\alpha$-SiS were simulated, respectively. We found that when the two O atoms attached to neighboring Si atoms, the value of the S-Si-O bond angle towards the other O atom (120.2°) is a little lager than the angle on the other side (111.0°), as shown in Fig. S1(a). However, the corresponding bond angles have the same value (115.9°) when the two O atoms are attached to spaced Si atoms, as shown in Fig. S1(b). Our DFT calculations show that $E_b$ per O atom in the structure shown in Fig. S1(a) is 0.06 eV smaller than that in the structure shown in Fig. S1(b). These results indicate that when O atoms are attached to neighboring Si atoms, they are too close to each other and will get repulsive interactions from the neighboring O atoms. As a result, in the fully optimized $\alpha$-SiS, the repulsion between the crowded O atoms leads to the reduced $E_b$ comparing to the isolated oxygen impurity. However, on the other hand, the repulsion between O atoms restricts the movements of all the O atoms and keeps a high thermodynamic stability of the whole structure.

## DETAILED PROJECTED DENSITY OF STATES FOR $\alpha$-SiSO

As demonstrated by the partial charge density associated with frontier states in the main manuscript, the valence band maximum (VBM) of $\alpha$-SiSO is dominated by $p_x$ orbitals from O atoms and the conduction band minimum (CBM) is dominated by a hybridization of $s$ and $p_y$ orbitals from Si and S atoms. To further verify this conclusion, detailed projected density of states (PDOS) plotting for different orbitals from each single element in $\alpha$-SiSO is presented in Fig. S2. From the PDOS plotting of oxygen we found that only $p_x$ orbitals of oxygen contributed to the total density of states (DOS) near the VBM, which can be easier distinguished from the inset of Fig. S2(a) for the amplified figure. From Fig. S2(b), (c) and the insets zoomed in near the CBM, we found that both $s$ and $p_y$ orbitals from Si and S contribute to the CBM. These results are consistent with what we discussed in the main manuscript.

## ELECTRONIC STRUCTURE OF UNSATURATEDLY OXIDIZED $\alpha$-SiS

The electronic band structure and the associated PDOS for monolayers of $\alpha_1$-SiSO$_{0.5}$, $\alpha_2$-SiSO$_{0.5}$ and $\alpha$-SiSO$_{0.25}$ are shown in Fig. S3. The corresponding equilibrium structures are shown in Fig. 6 of the main manuscript. Our DFT-PBE calculations show that all the three structures considered are semiconductors with indirect band gaps. The values of the band gaps for $\alpha_1$-SiSO$_{0.5}$, $\alpha_2$-SiSO$_{0.5}$ and $\alpha$-SiSO$_{0.25}$ are 1.25 eV, 2.27 eV and 1.39 eV, respectively. The VBM is located at $\Gamma$-Point and the CBM is located at $X$-Point for $\alpha_1$-SiSO$_{0.5}$. For $\alpha_2$-SiSO$_{0.5}$, the VBM is located at $X$-Point and the CBM is located between $\Gamma$-Point and $Y$-Point. For $\alpha$-SiSO$_{0.25}$, the VBM is located at $X$-Point and the CBM is located at $\Gamma$-Point.

* guanjie@seu.edu.cn

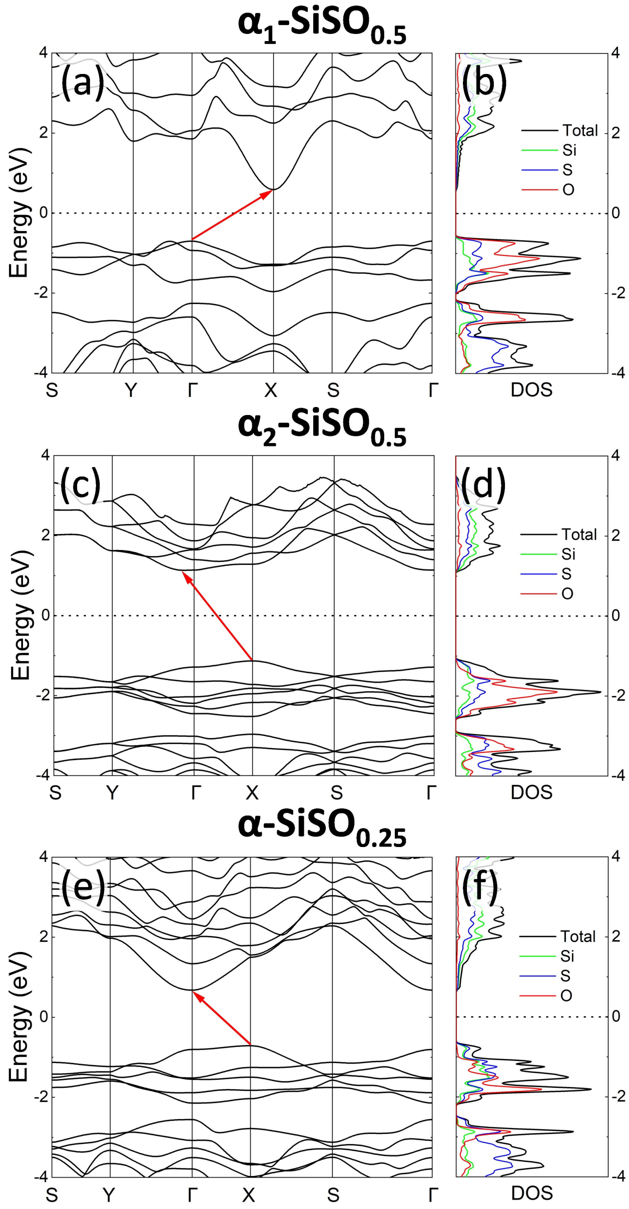


FIG. S3. Electronic band structures (left panel) and projected density of states (right panel) of (a), (b) $\alpha_1$-$SiSO_{0.5}$, (c), (d) $\alpha_2$-$SiSO_{0.5}$ and (e), (f) $\alpha$-$SiSO_{0.25}$. Indirect band gaps are shown by red arrows in (a), (c), (e). Contributions of electrons from different atoms in (b), (d), (f) are distinguished by color.
